# Supplementary material for: Addressable electron spin resonance using donors and donor molecules in silicon
Source: arXiv:1807.10290 ancillary file (2018-07-26)
Supplement: Supplementary file 1 [file paper_supp.pdf]

# Supplementary Materials: Addressable electron spin resonance using donors and donor molecules in silicon

Samuel J Hile,[1,*] Lukas Fricke,[1] Matthew G House,[1] Eldad Peretz,[1] Chen Chin Yi,[2] Yu Wang,[2] Matthew Broome,[1] Samuel K Gorman,[1] Joris G Keizer,[1] Rajib Rahman,[2] and Michelle Y Simmons[1,†]

[1] *Centre for Quantum Computation and Communication Technology (CQC$^2$T), School of Physics, University of New South Wales, Sydney 2052, Australia*

[2] *Network for Computational Nanotechnology, Purdue University, West Lafayette, IN, USA*

## I - MICROWAVE ANTENNA ALIGNMENT AND FIELD SIMULATIONS

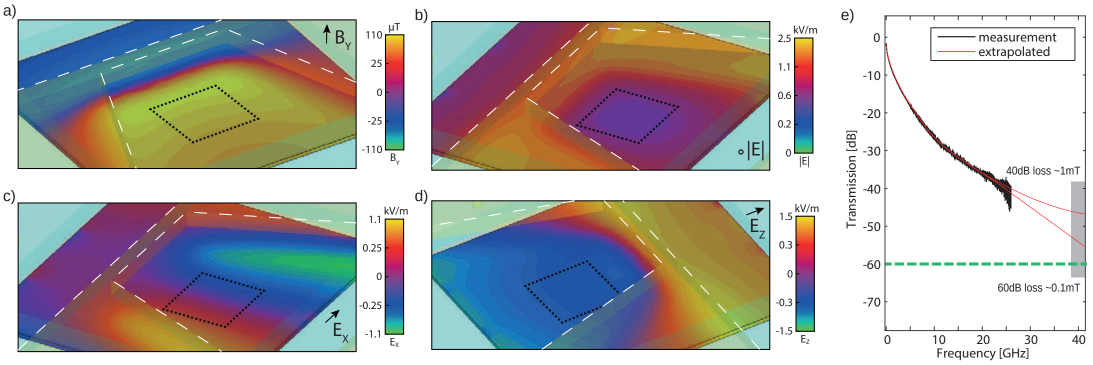


FIG. 1. **Finite element microwave field simulations.** (a) Magnetic field $B_Y$ and (b-d) electric field $|E|, E_X, E_Z$ simulations at 40GHz. The coloured panels plotting the fields are $2 \times 2\mu$m and lie 55nm below the silicon surface. White dashed lines indicate the position of the antenna. Grey boxes denote a $500 \times 500$nm target region where the ratio of magnetic to electric field is optimised. (e) Measured attenuation in the $\sim$ 2.5m long stainless steel coaxial cable used to transmit the microwave signal into our dilution refrigerator. Red lines extrapolate the loss to 40GHz

We performed finite element field simulations of the $B_1$ oscillating magnetic field produced by our antenna geometry prior to its fabrication, to allowing us to position the antenna to maximise the $B_1$ magnetic field at the donors' location and also minimise the stray AC electric field. The simulated magnetic field within a $2 \times 2\mu$m area 55nm below the end of the antenna is shown in Fig. 1(a), for an antenna driving frequency of 40GHz.

We aim also to minimise the E-field at the donor location, since large electric field fluctuations may lead to unintended ionisation of the donor during the spin resonance experiment, or adversely affect the SET charge sensor through photon-assisted tunnelling or charge pumping effects[1]. The electric field amplitude $|E|$ simulated for our antenna is shown in Fig. 1(b). Fig. 1(c) and (d) show the in-plane E-field components $E_X, E_Z$.

There is a 500nm $\times$ 500nm region of maximum magnetic field and minimal electric field, indicated by grey dotted lines – we take this as the target region in which we position the donor qubits.

For the simulation, the transmission line's TEM mode was excited with a nominal input power of 1mW. To produce realistic absolute field values in Fig. 1, we scale the simulation results commensurate with realistic losses in the full transmission line between the microwave signal generator and the on-chip antenna, which is dominated by $\sim$ 2.5m of stainless steel 2.2mm diameter (UT85) coaxial cable. We have measured the signal attenuation (at room temperature) in our coaxial cable up to 26GHz with a network analyser, as shown in in Fig. 1(e). Extrapolating the loss curve suggests we can expect on the order of $50 \pm 10$dB of attenuation at 40GHz. The use of stainless steel provides good thermalisation of the cable at the cost of significant signal loss, and we include an additional 10dB to account for further attenuation in the PCB launch adapter connecting the coaxial cable to coplanar waveguide. Overall this produces an estimate of 60dB total attenuation, which is the value we have used to scale the simulation outputs to the values shown in the field plots of Fig. 1(a-d). Based on this estimate, the expected $B_1$ field achievable within the target region is on the order of 0.1mT with a nominal input power of 1mW = 0dBm. Importantly, the electric fields we expect the antenna to generate are in the low kV/m range, orders of magnitude lower than typical DC electric fields in planar donor-defined devices which are on the order of several MV/m, and thus should not lead to unwanted electron tunnelling during an ESR pulse.

## II - INITIALISATION AND READOUT PULSE SEQUENCE

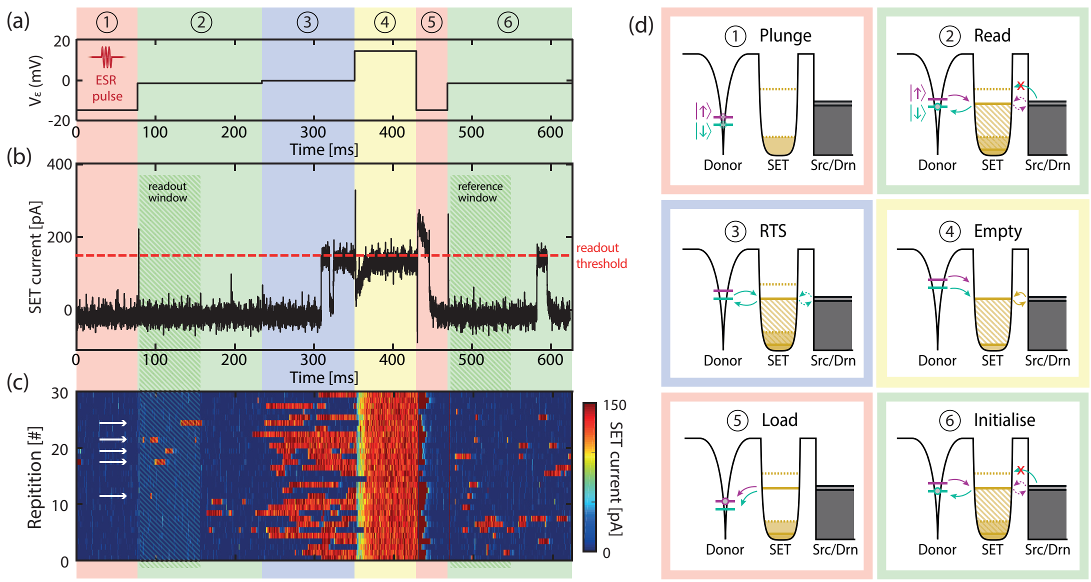


FIG. 2. **Pulse protocol incorporating continuous interleaved monitoring of charge stability.** (a) A six stage pulsed voltage sequence defined on the detuning axis $V_\epsilon$, as a function of time for spin resonance measurements of the 1P qubit, and (b) a sample SET current trace for a single-shot spin manipulation, readout, and re-initialisation sequence. The spin is determined to be $|\uparrow\rangle$ if the current trace exceeds the readout threshold level within the readout window as indicated. This sample shows a $|\downarrow\rangle$ outcome. (c) 30 single-shot current traces, 5 of which are identified as $|\uparrow\rangle$ outcomes, as indicated by white arrows. (d) Electrochemical potential diagrams corresponding to each of the six stages: ① plunge, ② read, ③ RTS, ④ empty, ⑤ load, ⑥ initialise.

To ensure reliable measurements in the presence of low frequency charge fluctuations, we continuously monitor two feedback signals, extracted from the mean value of our SET charge sensor signal during auxilliary phases within a 6 phase pulse sequence. This monitoring effectively prevents systematic errors in the spin readout process which would arise if the working point drifts by a significant fraction of the Zeeman energy ($\sim 0.2$mV) during a measurement. In Fig. 2 we present the timing sequence used for the 1P electron experiment, optimised to its tunnel rate. The sequence for the 2P electron is equivalent but with different pulse timings.

Fig. 2(a) shows the input voltage offset along the detuning ($\epsilon$) axis, and Fig. 2(b) shows an exemplary output trace of the SET current during one repetition of the sequence. Thirty additional example traces are shown in Fig. 2(c), illustrating typical statistics. The steps executed are as follows, and each configuration is illustrated in Fig. 2(d).

① **Plunge:** The donor potential is lowered far into Coulomb blockade as shown in Fig. 2(d-1) for the application of an ESR microwave pulse, which occurs at a time ($\sim$ 40ms) midway through this stage.

② **Read:** The donor Zeeman state potentials are raised to straddle the SET Fermi level, enabling spin readout. The probability that a current 'blip' is due to a $|\uparrow\rangle$ electron tunnelling to the SET (pink arrow in Fig. 2(d-2)) decays exponentially with increasing time. However, the probability for a thermally excited $|\downarrow\rangle$ to tunnel and cause an erroneous blip remains constant in time, therefore to maximise the readout fidelity we restrict the spin readout discrimination routine so that only blips occurring in the first 76ms are assigned as $|\uparrow\rangle$.

③ **RTS:** The donor potential is raised slightly above the read level such that the spin down state is resonant with the SET Fermi level as indicated in Fig. 2(d-3). Here we observe a random telegraph signal (RTS) due to electrons tunnelling back and forth between the donor and SET. By measuring the average value of the SET current $\langle I\rangle_3$ during this phase, over many repetitions (typically $>$ 200 single shots), we obtain a feedback signal used to adjust gate voltages and recover a proper working point.

④ **Empty:** The donor potential is raised far above the SET Fermi level, causing the electron to tunnel to the SET. The SET current is expected to be high for this phase, with the SET Fermi level resonant with source and drain

Fermi levels as shown in Fig. 2(d-4). We monitor the average SET current value in this phase $\langle I \rangle_4$ as a second feedback signal, and if it falls below the expected value, we trigger a realignment procedure to re-calibrate our voltage working point.

⑤ **Load:** The donor potential is lowered far below the SET Fermi level, loading an electron with random spin as shown in Fig. 2(d-5)

⑥ **Initialise:** The donor potential is held at the same read position as for step ②, and the presence of current blips within a 'reference window' is used to produce a reference spin-up probability. This reference value should remain consistent throughout the course of a spin resonance experiment, because it is based on the measurement of randomly loaded spins independent of the effect of any applied ESR microwave pulse during phase ①. At the end of this reference readout phase the spin is deterministically initialised $|\downarrow\rangle$ with high probability, as indicated by the blue arrow in Fig. 2(d-6).

The continuous monitoring of the feedback signals $\langle I \rangle_3$ and $\langle I \rangle_4$ provide real-time information allowing the automated system to determine when low frequency charge noise causes the SET or donor potentials to drift. Execution of an automated realignment procedure corrects for the random drift, keeping the system fixed at a working point where high fidelity spin readout may be continuously carried out.

## III - STATIC ELECTRIC FIELD SIMULATIONS

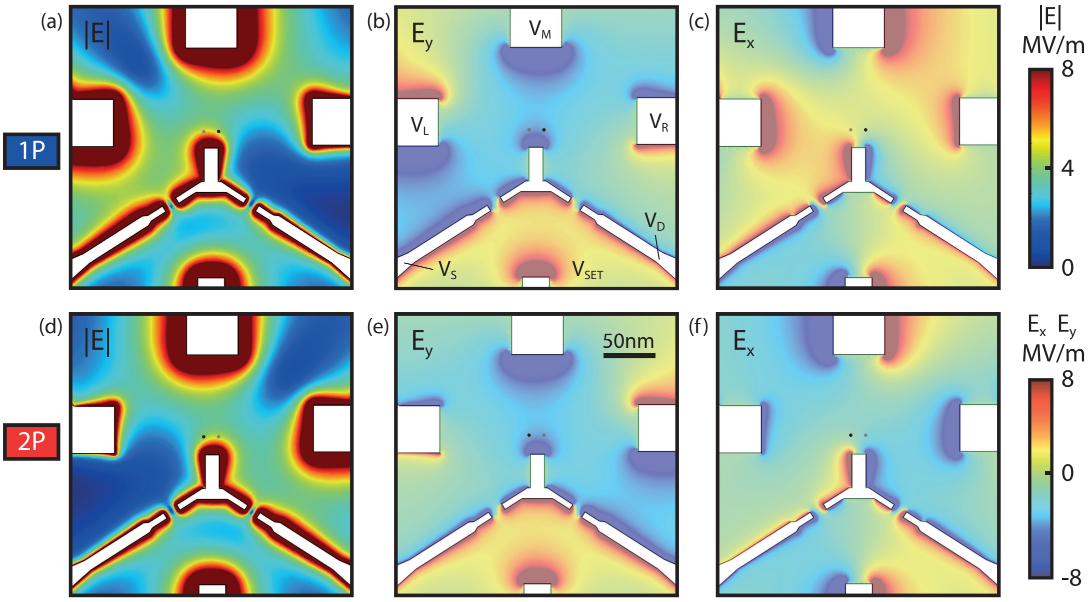


FIG. 3. **Electric fields at the 1P and 2P qubit operating points.** (a,b,c) Electric field magnitude, y-component, and x-component as simulated for the gate voltage configuration corresponding to the 1P qubit (d,e,f) Electric field magnitude, y-component, and x-component as simulated for the gate voltage configuration corresponding to the gate voltages used for the 2P qubit. Colour-bars are provided separately for the field magnitude ($[0-8]$MV/m) and in-plane field components ($[-8, 8]$MV/m), the qubit positions are marked as black dots, and applied voltage labels are shown in (b).

Knowing the voltages applied to the gates, we estimated the electric field present at each donor site using a simple finite-element field solver (*Comsol Multiphysics*), modelling the P doped conducting structures as perfect conducting sheets within an infinite block of silicon. The results of the simulation are shown in Fig. 3 and Table I.

## IV - 1P NUCLEAR SPIN DYNAMICS

In order to examine the cause of asymmetric peak-heights in the 1P resonance spectrum, Fig. 4(a) and (b) compare the 1P spectra observed at 1.35 and 1.55T. Solid dots indicate the overall average spin-up fraction $f_\uparrow$, obtained by

| Parameter | Right qubit (1P) | Left qubit (2P) |
|---|---|---|
| $V_S$ (mV) | 2 | 2 |
| $V_D$ (mV) | 0 | 0 |
| $V_L$ (mV) | 730 | 43 |
| $V_M$ (mV) | 800 | 800 |
| $V_R$ (mV) | −50 | 650 |
| $V_{SET}$ (mV) | 600 | 600 |
| $\|E\|$ (MV/m) | 4.5±0.1 | 4.3±0.1 |
| $E_x$ (MV/m) | 0.9±0.2 | −0.5±0.2 |
| $E_y$ (MV/m) | −4.4±0.1 | −4.3±0.1 |

TABLE I. Gate settings and resultant E-field estimates at the two qubit working points: the E-field is numerically computed by solving the Poisson equation with boundary conditions derived from the gate settings. The uncertainty in E-field values are based on a positional uncertainty for the qubits of $\sim$ 1nm.

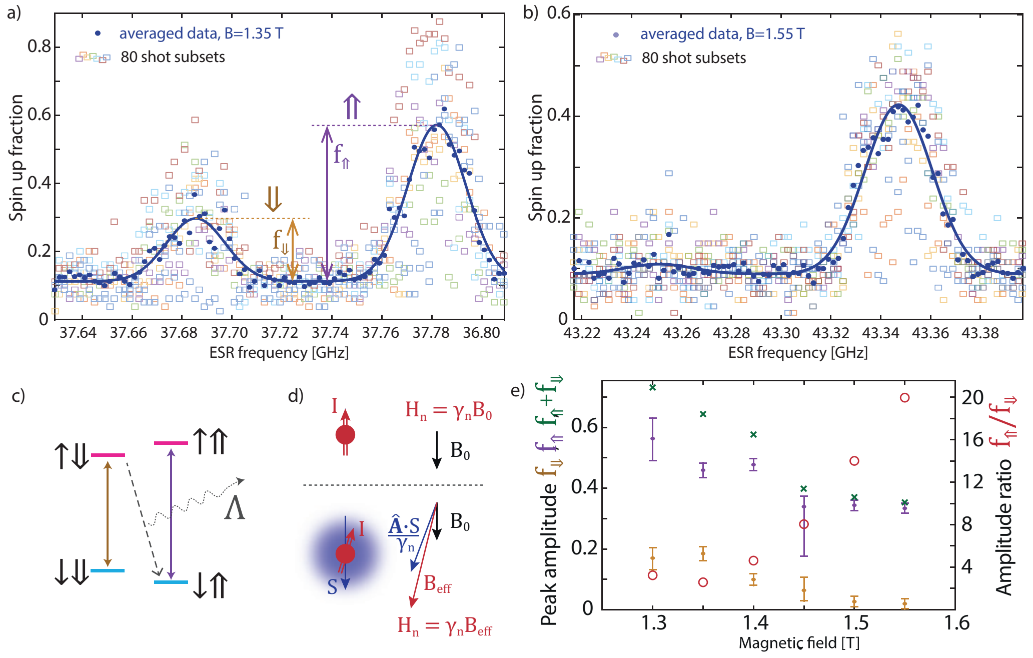


FIG. 4. **Development of asymmetry in the 1P hyperfine spectrum with increasing magnetic field** (a) Average spin up probability at 1.35T, and short time binning of the same data set into 80 shot bins for each frequency. Coloured squares exhibit non-uniform scatter, departing from the average significantly at the resonance conditions, and indicating observation of nuclear dynamics at the binning timescale of $\sim$ 50s (b) Similar data for 1.55T. The left peak is notably suppressed due to a nuclear-electron flip-flop process, releasing the energy difference as a phonon. (c) Schematic of the flip-flop cross relaxation mechanism, emitting energy $\Lambda$ to the phonon bath while conserving spin. (d) Ionisation shock may flip the nuclear spin when its effective magnetic field is non-adiabatically altered by the addition or removal of an electron. The anisotropic hyperfine interaction tilts the hyperfine field $\hat{A} \cdot S$ (e) Evolution of the two resonance peak amplitudes (tan, purple) as defined by arrows in (a), along with their sum (green) and ratio (red) as a function of magnetic field, displaying the gradual suppression of the low frequency resonance as the nuclear spin pumping process becomes more efficient.

averaging over several repeated frequency sub-scans. In each scan the order of points is randomised to average out any time dependent measurement artefacts. The individual sub-scan results are shown here, each coloured square marker showing $f_\uparrow$ for 80 sequential single-shot measurements within a single (50 second) time-bin. By binning in this way we reveal further information about the nuclear spin dynamics.

Because $f_\uparrow$ is not consistent for data-points at the same frequency but in different time bins, we infer that with this time binning we approach the timescale of nuclear spin flips, preferentially sampling either the nuclear $|\Uparrow\rangle$ or $|\Downarrow\rangle$ state rather than averaging equally over the two. Limited by the tunnel rate ($\sim$ 10ms), we are unable to explore the time dynamics on shorter timescales for this donor.

The nuclear spin polarisation is attributed to an inelastic electron-nuclear flip-flop process, as disscussed in the

main text and illustrated in Fig. 4(c).

Repopulation of the nuclear $|\Downarrow\rangle$ has been observed[2] and attributed to a process described as *ionisation shock*. Here the effect of projecting the nuclear spin onto a time varying quantisation axis when loading and unloading electrons will result in a non-adiabatic change of eigenstate with low but non-zero probability. We illustrate the concept in Fig. 4(d), where the upper panel shows the nuclear spin $I$ aligned (in this case anti-parallel) to the external field $B_0$ in the absence of an electron. With a Hamiltonian consisting only of the nuclear Zeeman term, $|\Downarrow\rangle$ and $|\Uparrow\rangle$ are perfect eigenstates. The lower panel shows the situation where the donor is occupied by an electron of spin state $S$. Here, the states $|\downarrow\Uparrow\rangle$ and $|\uparrow\Downarrow\rangle$ are not perfect eigenstates of the two spin Hamiltonian containing now a hyperfine interaction term. The eigenstates for these two spin anti-parallel states are properly described as:

$$\left|\widetilde{\downarrow\Uparrow}\right\rangle = \cos(\eta/2)\,|\downarrow\Uparrow\rangle - \sin(\eta/2)\,|\uparrow\Downarrow\rangle \tag{1}$$

$$\left|\widetilde{\uparrow\Downarrow}\right\rangle = \cos(\eta/2)\,|\uparrow\Downarrow\rangle + \sin(\eta/2)\,|\downarrow\Uparrow\rangle \tag{2}$$

$$\tan(\eta) = \frac{A}{(\gamma_e + \gamma_n)B_0} \tag{3}$$

While the mixing angle $\eta$, describing the degree of approximation in assuming the simple product states as eigenstates (at a field of $B_0 = 1.55$T and hyperfine coupling $A = 96.5$MHz) is only $\sim 2.2 \times 10^{-9}$, the misalignment of eigenstates may be enhanced by the presence of an anisotropic component to the hyperfine interaction, which is in general defined by a tensor $\hat{A}$. The diagonal terms dominate, meaning that it is normally sufficient to consider a scalar approximation of $A$ in what is called the contact hyperfine interaction. Small off-diagonal tensor components, arising from anisotropy in the electron wavefunction for instance due to a non-zero electric field in the device, would allow the nuclear spin to experience an effective magnetic field component $(\hat{A} \cdot S)/\gamma_n$ that is not parallel to the external $B_0$ field, although the electron spin $S$ is. By a combination of the two effects (non-zero mixing angle $\eta$, and anisotropic hyperfine $\hat{A}$) the quantisation axis for the nuclear spin changes instantaneously as indicated in the sketch of Fig. 4(d) by $B_0$ and $B_{\text{eff}}$ whenever the donor is ionised during the readout, feedback and initialisation sequence. Precession around these constantly switching axes allows the nuclear spin to flip back to $|\Downarrow\rangle$, providing an explanation for why we do not observe permanent occupation of the $|\Uparrow\rangle$ state, and complete supression of the lower frequency resonance peak, since the nuclear $T_1$ relaxation time for phosphorus donors is known to be on the order of thousands of seconds at low temperature[3].

Further to the asymmetry in the amplitude of the two resonances, we observe a decrease in amplitude of both resonances at higher fields, as shown in Fig. 4(e), which plots the amplitudes of the two resonance peaks for $|\Downarrow\rangle$ and $|\Uparrow\rangle$ as a function of $B_0$. Both peaks lose intensity with increasing magnetic field, and the lower line disappears almost completely within the noise floor at $f_0$ at $B_0 = 1.55$T. The reduction in overall spin-up fraction (the sum of up and down amplitudes, shown as green crosses) may suggest that the adiabatic passage is becoming non-adiabatic due to higher attenuation of the microwave signal at higher frequency, and consequently a reduced $B_1$ field strength. The change in *relative* peak intensity $f_{\Uparrow}/f_{\Downarrow}$ however, plotted with red ring markers and on the right side axis of Fig. 4(e), suggests a process that is Zeeman energy dependent, such as the reverse of the 'flip-flop' cross-relaxation process discussed above. We were unable to measure at fields below $\sim 1.3$T, because the Zeeman energy becomes comparable to the thermal energy of the system. If there are thermal phonons available with energy equal to the difference in $|\downarrow\Uparrow\rangle$ and $|\uparrow\Downarrow\rangle$ states, as is evidently the case in our device for the smaller magnetic field values, phonon absorption can mediate a 'flop-flip' transition, the reverse of the 'flip-flop' shown in Fig. 4(c). As the field increases, and the Zeeman energy becomes larger, the rates of the two phonon mediated transitions diverge and the weighting of the two peaks becomes more asymmetric.

## V - 2P NUCLEAR SPIN DYNAMICS

In order to investigate the lack of asymmetry in our observed 2P spectrum, we again analyse the spectrum at different magnetic fields. In Fig. 5(a) at $B_0 = 1.35$T and (b) at $B_0 = 1.55$T we see an equal probability for each of the 4 nuclear spin subspaces, and observe no strong magnetic field dependence of the peak distribution, as shown in Fig. 5(c) which plots the three amplitudes as a function of $B_0$. Time-binning of our measurement similar to Fig. 4 does not reveal any statistically significant variation in populations over time, so we instead perform an experiment where we repeatedly initialise an electron $|\downarrow\rangle$, excite the central resonance peak with an adiabatic passage pulse, and measure the electron spin, 40 000 times. This experiment allows us to determine whether the nuclear spin state is stable over the timescale of a single shot measurement sequence, which for the 2P qubit is 42ms. The outcome is

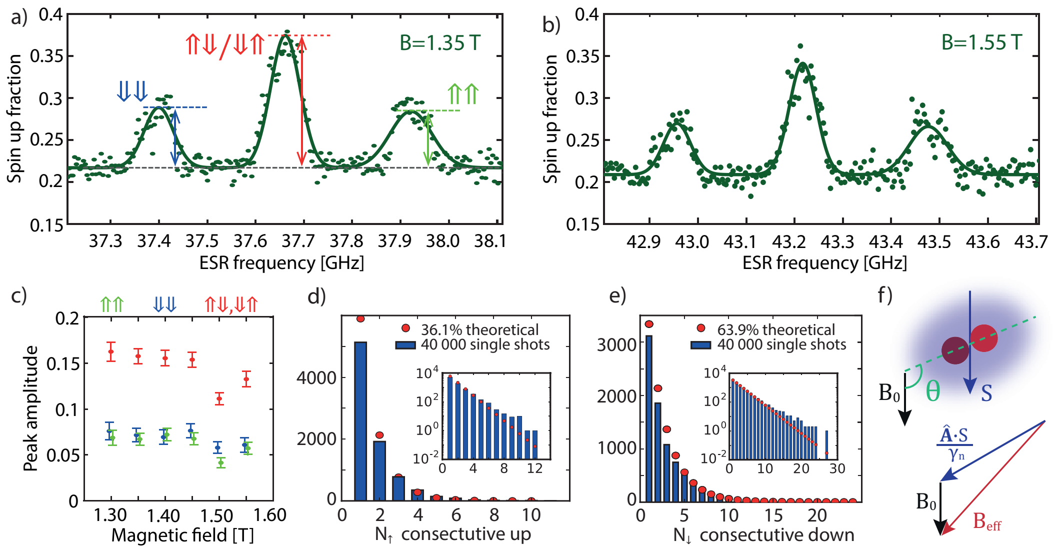


FIG. 5. **Populations of the 2P nuclear states remain independent of the magnetic field** (a)Average electron spin up probability taken from 2000 single shot measurements at 1.35T, with peak amplitudes marked. (b) Similar data for 1.55T, with no significant shift in distribution of the peaks. (c) The three extracted peak heights for magnetic field values from 1.3 to 1.55T, showing no significant trend in the corresponding peak amplitudes. (d) Statistical analysis of the nuclear spin dynamics. We plot a histogram (in blue) of the number of times we observe N successive spin-up outcomes before the first spin-down, using a set of 40 000 single shot measurements all taken at the central resonance peak after an adiabatic inversion pulse. The red markers are the calculated distribution expected for a perfectly Markovian system (with no memory of the previous state). Inset plots the same histogram on a logarithmic scale for clarity. (e) a similar histogram of the count of N successive spin-down outcomes before the first spin-up, using the same data set.

shown in Fig. 5(d), where we plot a histogram of the number of times we observe N successive spin-up outcomes before the first spin-down reading. This is compared with a calculated Markovian histogram produced by a series of completely independent outcomes with the same overall probability of observing spin-up (the red dots). The inset plots the same statistics on a logarithmic scale. Fig. 5(e) uses the same data set to plot the equivalent histogram of N successive spin-downs. We see very good agreement with the Markov model, showing that indeed the nuclear state has no long term memory and is randomised on the timescale of a single shot. This therefore indicates that the lack of state polarisation is likely due to an enhancement in the *ionisation shock* mechanism. This can be understood in the context of a 2P donor molecule by noting that the hyperfine tensor **D** is likely to be more highly anisotropic than in the single donor case, since the total electron wavefunction is in general not spherically symmetric.

We illustrate the effect of anisotropy in Fig. 5(f). In the molecular frame, where the z-axis is defined by a vector passing through the two donor atom sites (green dashed line in Fig. 5(f)), the full hyperfine tensor for each donor individually can be expressed in a cylindrically symmetric form:

$$(A\mathbf{I} + \mathbf{D}) = \begin{pmatrix} A-d & 0 & 0 \\ 0 & A-d & 0 \\ 0 & 0 & A+2d \end{pmatrix} \tag{4}$$

$$A = \frac{2\gamma_e \gamma_N \mu_0}{3} |\Psi(r=0)|^2 \tag{5}$$

$$d = \frac{\gamma_e \gamma_N \mu_0}{10\pi} \left\langle \frac{3\cos^2\theta - 1}{r^3} \right\rangle \tag{6}$$

Here the terms $A$ and $d$ represent respectively the contact and dipolar components of the hyperfine interaction, where $r$ is the distance from the atom to a position within the extent of the assumed axially symmetric electron wavefunction. The right hand side of Eq. (6) averages over the entire wavefunction, and $\theta$ defines the angle between the molecular axis and $B_0$. When this tensor is transformed into the frame defined by the $B_0$ quantisation axis, for large angles $\theta$ there will be significant off-diagonal terms, tilting the effective total magnetic field $B_{\text{eff}}$ experienced by each nuclear spin in the presence of an electron. This tilt will (in general) be off-axis from the vector of $B_0$ which is the only

magnetic field seen by the nucleus when ionised. This means the true eigenstates for the two charge states are less alike, and we would therefore expect to see enhanced nuclear spin randomisation by *ionisation shock*, consistent with our observations.

## VI - ATOMISTIC TIGHT BINDING MODELLING

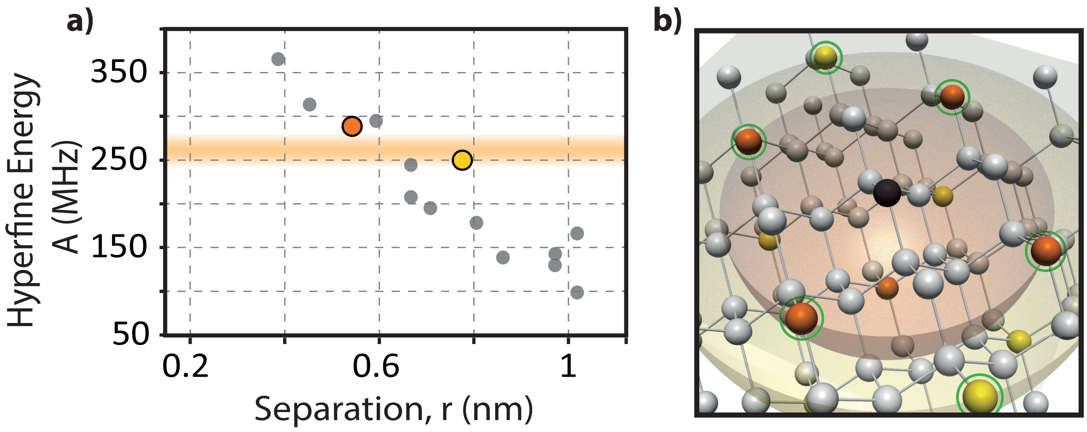


FIG. 6. **Intrinsic hyperfine energies for different donor configurations of a 2P molecule.** (a) Simulated Hyperfine interaction energy $A$, for atomic configurations of a 2P quantum dot with donor separation less than 1nm, and including out-of-plane configurations with upto a 2 monolayer vertical offset between the two donor atoms. In-plane configurations consistent with our measurement are coloured orange and yellow. (b) 3D schematic showing the layout of the silicon crystal in the fabrication plane and several monolayers below.

| Distance (nm) | Sep. vector | Multiplicity | Hyperfine (MHz) |
|---|---|---|---|
| 0.235[a] | (1,1,1) | 4 | 229 |
| 0.384 | (2,2,0) | 12 | 366 |
| 0.450 | (3,1,1) | 12 | 314 |
| 0.543 | (4,0,0) | 6 | 287 |
| 0.591 | (3,3,1) | 12 | 295 |
| 0.665 | (4,2,2) | 12 | 244 |
| 0.665[b] | (4,2,2) | 12 | 207 |
| 0.705 | (5,1,1) | 12 | 195 |
| 0.768 | (4,4,0) | 12 | 250 |
| 0.803 | (5,3,1) | 12 | 179 |
| 0.859 | (6,2,0) | 24 | 139 |
| 0.970 | (7,1,1) | 12 | 130 |
| 1.016 | (6,4,2) | 12 | 99 |
| 1.016 | (6,4,2) | 12 | 164 |

[a] Not shown on plot. Nearest neigour sites form electrically inactive P-P bonds.
[b] There are two non-identical configurations at 0.665nm (and at 1.016nm) given the tetrahedral bond pattern in silicon.

TABLE II. Equivalence classes of donor-donor interatomic separation vectors, specified in units of $1/4a$. The multiplicity of each class represents the number of equivalent atoms at the same distance.

Simulations to determine the hyperfine interaction energy based on donor configuration and electric field were carried out with the NEMO-3D [4, 5] framework. The model encompasses numerical computation of electronic bandstructure, potential, charge density and other physical properties based on benchmarking by self-consistently solving the Schrodinger and Poisson equations in a domain encompassing several million atoms, where the wavefunction for each atom is described in a $sp^3d^5s^*$ spin-resolved (therefore 20 states) tight-binding orbital basis.

The geometrical layout for the full set of out-of-plane configurations are displayed in Fig. 6, considering up to 2 monolayers of vertical displacement between the two donors. Fig. 6(a) plots the full set of computed $A$ values for separation $< 1$nm. The layout of atoms in the silicon lattice is sketched in Fig. 6(b), with the in-plane configurations consistent with our measured hyperfine splitting coloured yellow and orange.

## VI - TIGHT BINDING MODEL OF 2P HYPERFINE STARK SHIFT

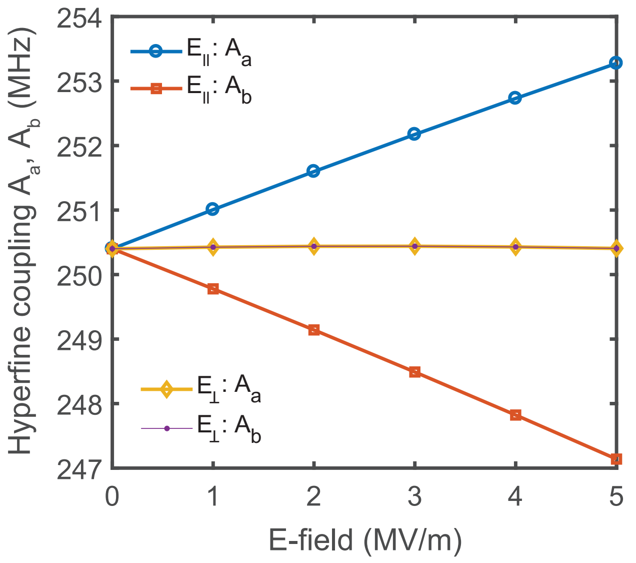


FIG. 7. **Computed Stark shift of the hyperfine coupling.** For two donors $a$ and $b$ separated by 0.768nm , the Stark shifted hyperfine coupling under an applied electric field either perpendicular to the molecular axis ($E_{\perp}$) or with an in-plane electric field, with a component parallel to the molecular axis ($E_{\|}$). The maximum ESR transition frequency shift corresponds to the difference of the blue and orange curves $\sim$ 6MHz.

In Fig. 7, we show the variation of the hyperfine couplings of a 2P cluster as a function of electric field as computed from atomistic tight-binding. A lateral in-plane electric field can detune the wavefunction between the two donors and produce unequal charge densities at the two donor sites. This results in a linear Stark shift of the hyperfine couplings, which will manifest as a splitting of the central ESR transition peak of a 2P cluster into two [6]. However, even for a field as large as 5MV/m, we find the difference in the two hyperfine couplings amount to $\sim$ 6MHz, which is far smaller than the measured 72MHz of linewidth broadening of the central peak, and is therefore, not resolvable in our experiment. Fig. 7 also shows that the Stark shift due to a vertical electric field is almost negligible compared with the lateral Stark effect. The vertical field actually produces a very weak quadratic Stark shift due to a tightly bound 2P wavefunction. Therefore, the major variations in the hyperfine couplings in terms of transition peaks and their separations result from the number and location of the donors. Electric fields produce a minor perturbation to these values.

* samhile@gmail.com
† michelle.simmons@unsw.edu.au

[1] E. Kawakami, P. Scarlino, L. R. Schreiber, J. R. Prance, D. E. Savage, M. G. Lagally, M. A. Eriksson, and L. M. K. Vandersypen, Applied Physics Letters **103**, 132410 (2013).
[2] J. J. Pla, K. Y. Tan, J. P. Dehollain, W. H. Lim, J. J. Morton, F. A. Zwanenburg, D. N. Jamieson, A. S. Dzurak, and A. Morello, Nature **496**, 334 (2013).
[3] J. J. Morton, A. M. Tyryshkin, R. M. Brown, S. Shankar, B. W. Lovett, A. Ardavan, T. Schenkel, E. E. Haller, J. W. Ager, and S. A. Lyon, Nature **455**, 1085 (2008).
[4] G. Klimeck, F. Oyafuso, T. B. Boykin, R. C. Bowen, and P. von Allmen, Comput. Model. Eng. Sci **3**, 601 (2002).
[5] S. Steiger, M. Povolotskyi, H.-H. Park, T. Kubis, and G. Klimeck, IEEE Transactions on Nanotechnology **10**, 1464 (2011).
[6] H. Büch, S. Mahapatra, R. Rahman, A. Morello, and M. Y. Simmons, Nature Communications **4**, 2017 (2013).
